# Supplementary material for: SWE-Bench+: Enhanced Coding Benchmark for LLMs
Source: arXiv:2410.06992 source file (2024-10-10)
Supplement: Supplementary file 1 [file appendix.tex]

\section{Appendix}

\begin{figure}[H]
    \vspace{-3mm}
    \centering
    \includegraphics[width=1\textwidth, trim={0 1cm 0 1cm}, clip]{pattern_distribution.eps} % Adjust trim values to crop whitespace
    \caption{Distribution of patterns across different models\song{reduce the height of this figure, takes too much space, also update the patterns} \reem{patterns are correct}}
    \label{patterns_distribution_image}
\end{figure}
